# Supplementary material for: Multi-scale Anomaly Detection for Big Time Series of Industrial Sensors
Source: arXiv:2204.08159 source file (2022-04-18)
Supplement: Supplementary file 1 [file appendix.tex]

\begin{figure*}[htbp]
    \centering
    \vspace{-40pt}
    \subfigure[AUC score of \method WO PCA.]{
        \label{fig:pca_wo_auc}
    \begin{minipage}{0.31\linewidth}
    \includegraphics[width=\linewidth]{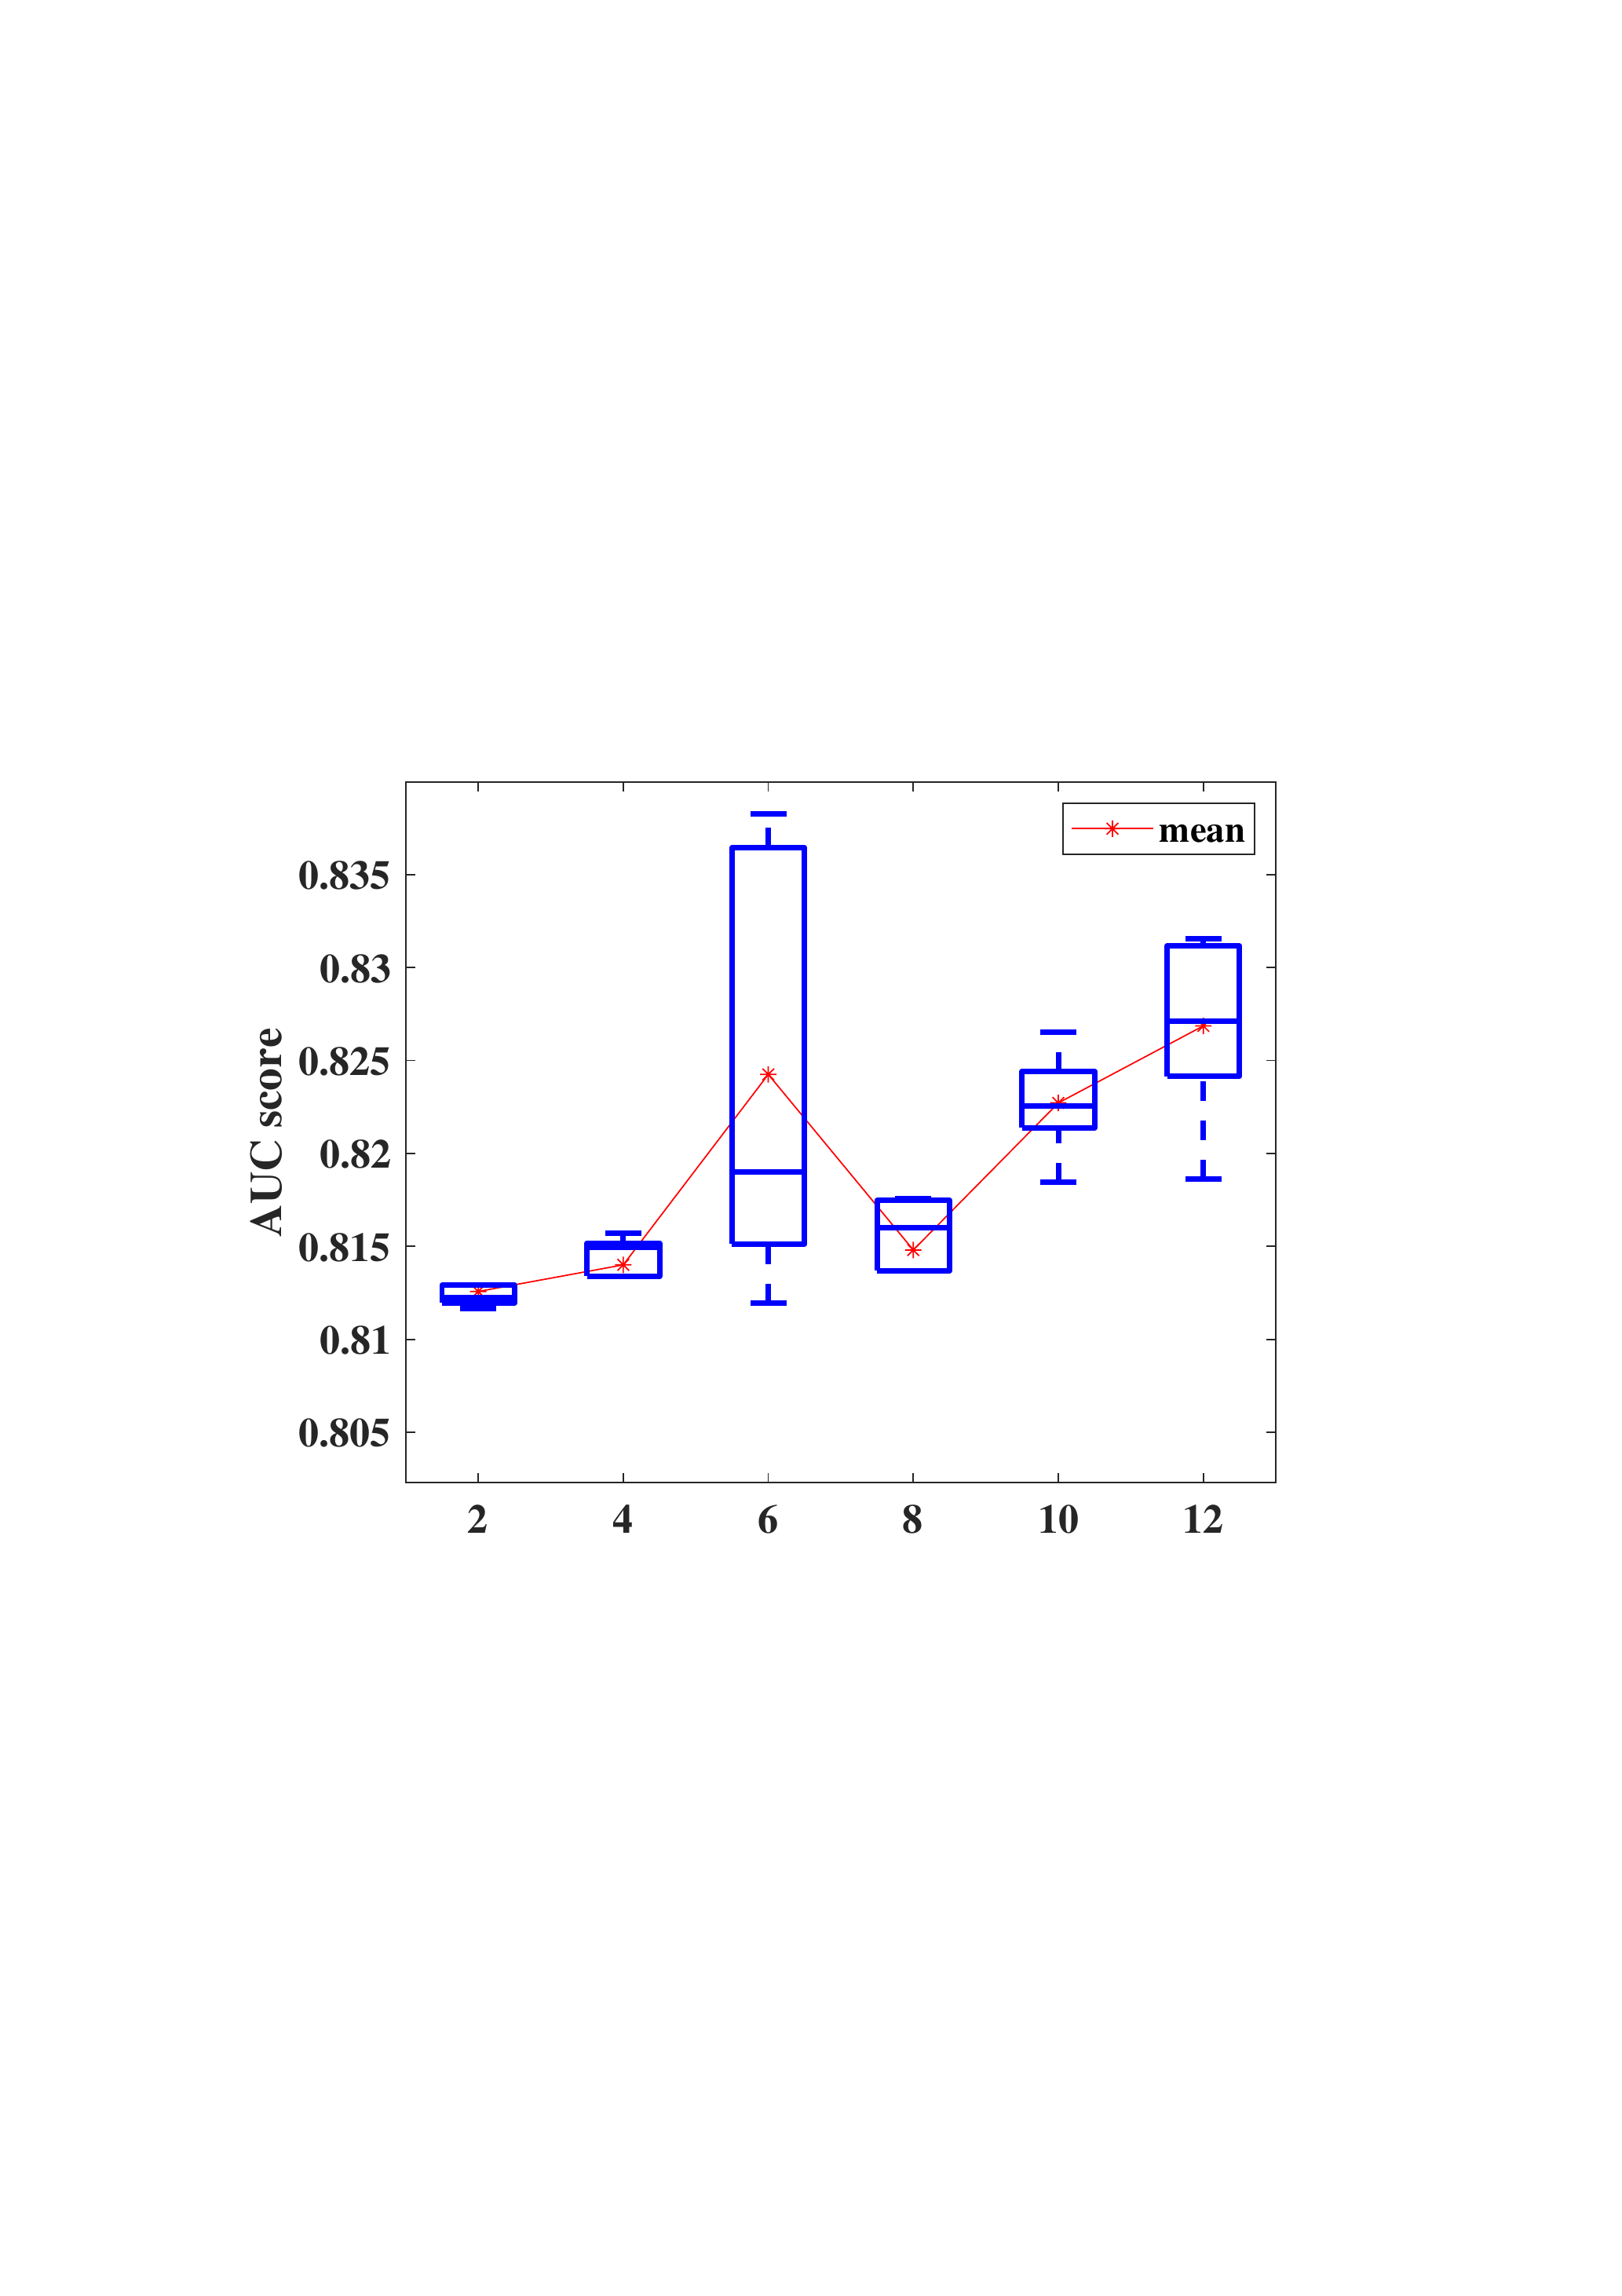}
    \end{minipage}
    }
    \subfigure[Ideal F1 score of \method WO PCA.]{
        \label{fig:pca_wo_f1}
    \begin{minipage}{0.31\linewidth}
    \includegraphics[width=\linewidth]{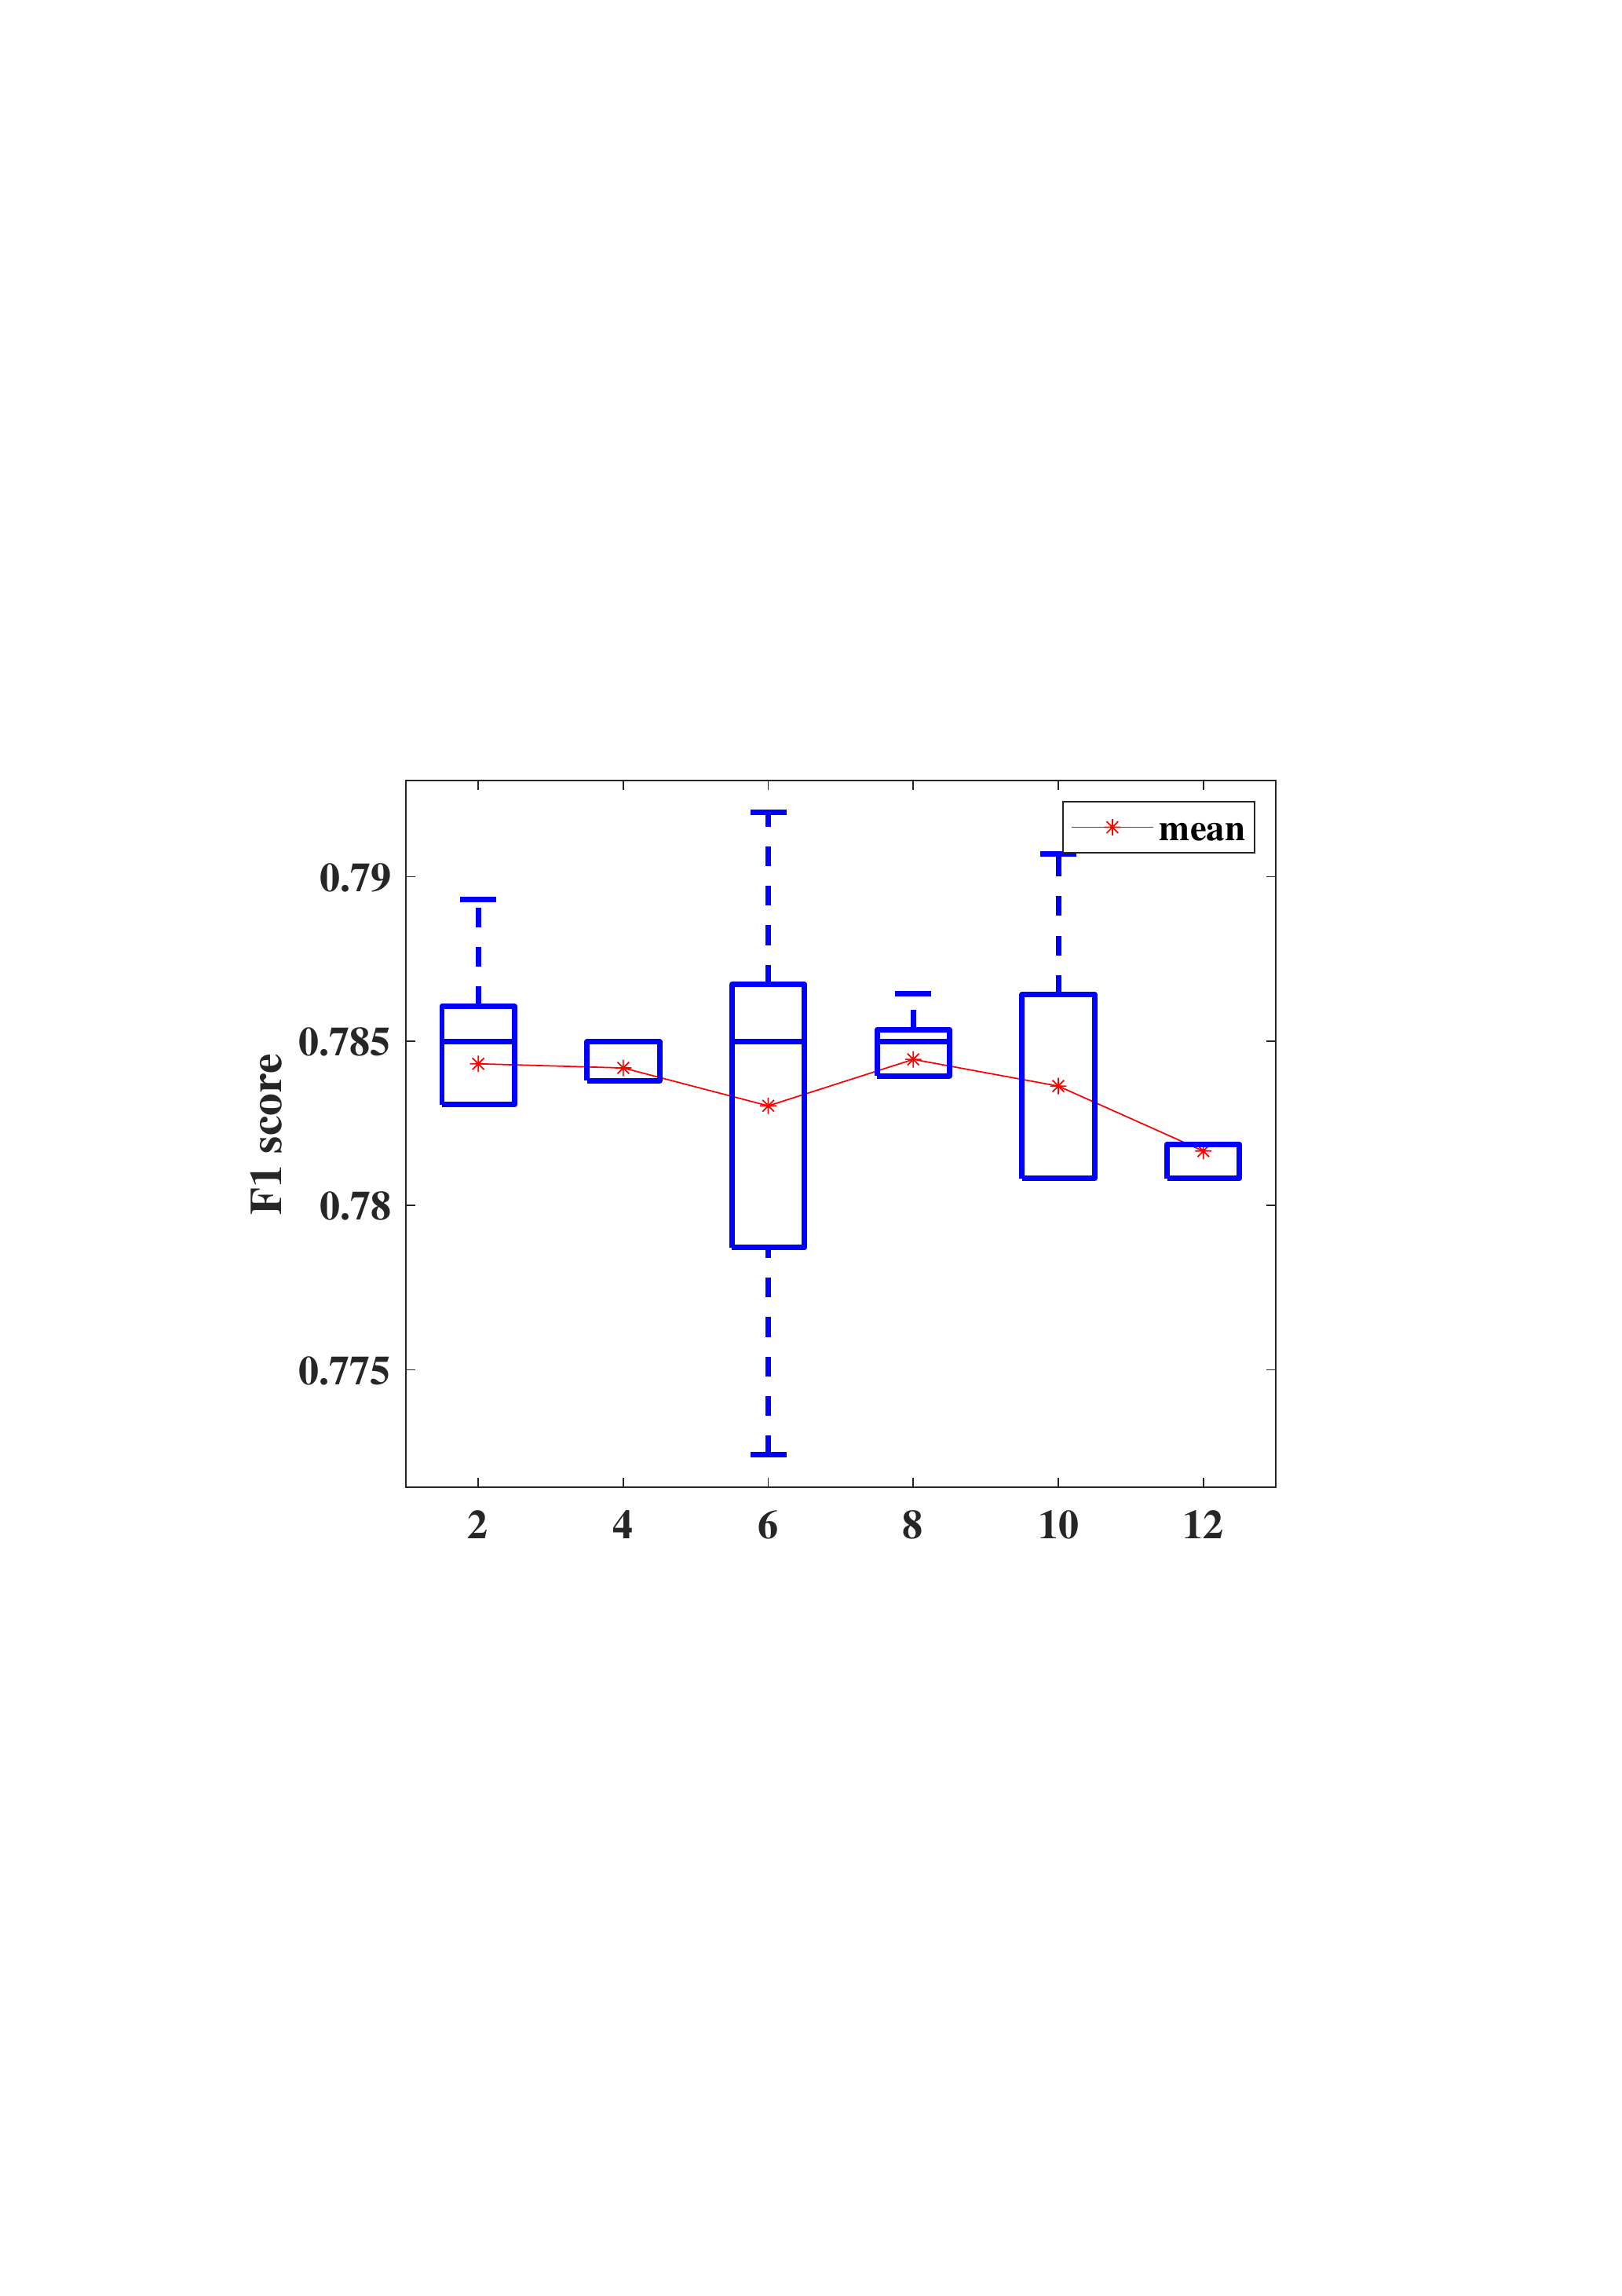}
    \end{minipage}
    }
    
    \caption{AUC and ideal F1 score of lambda experiments and dimension reduction. 
    Model with PCA uses PCA to compress dimensions while model without PCA directly reduces size of hidden neurons. 
    Numbers on x-axis stand for dimensions being reduced to.}
\end{figure*}

\begin{figure*}[htbp]
    \subfigure[Algorithm runs in linear time.]{
        \label{fig:time_consumption}
        \begin{minipage}{0.28\linewidth}
            \includegraphics[width=\linewidth]{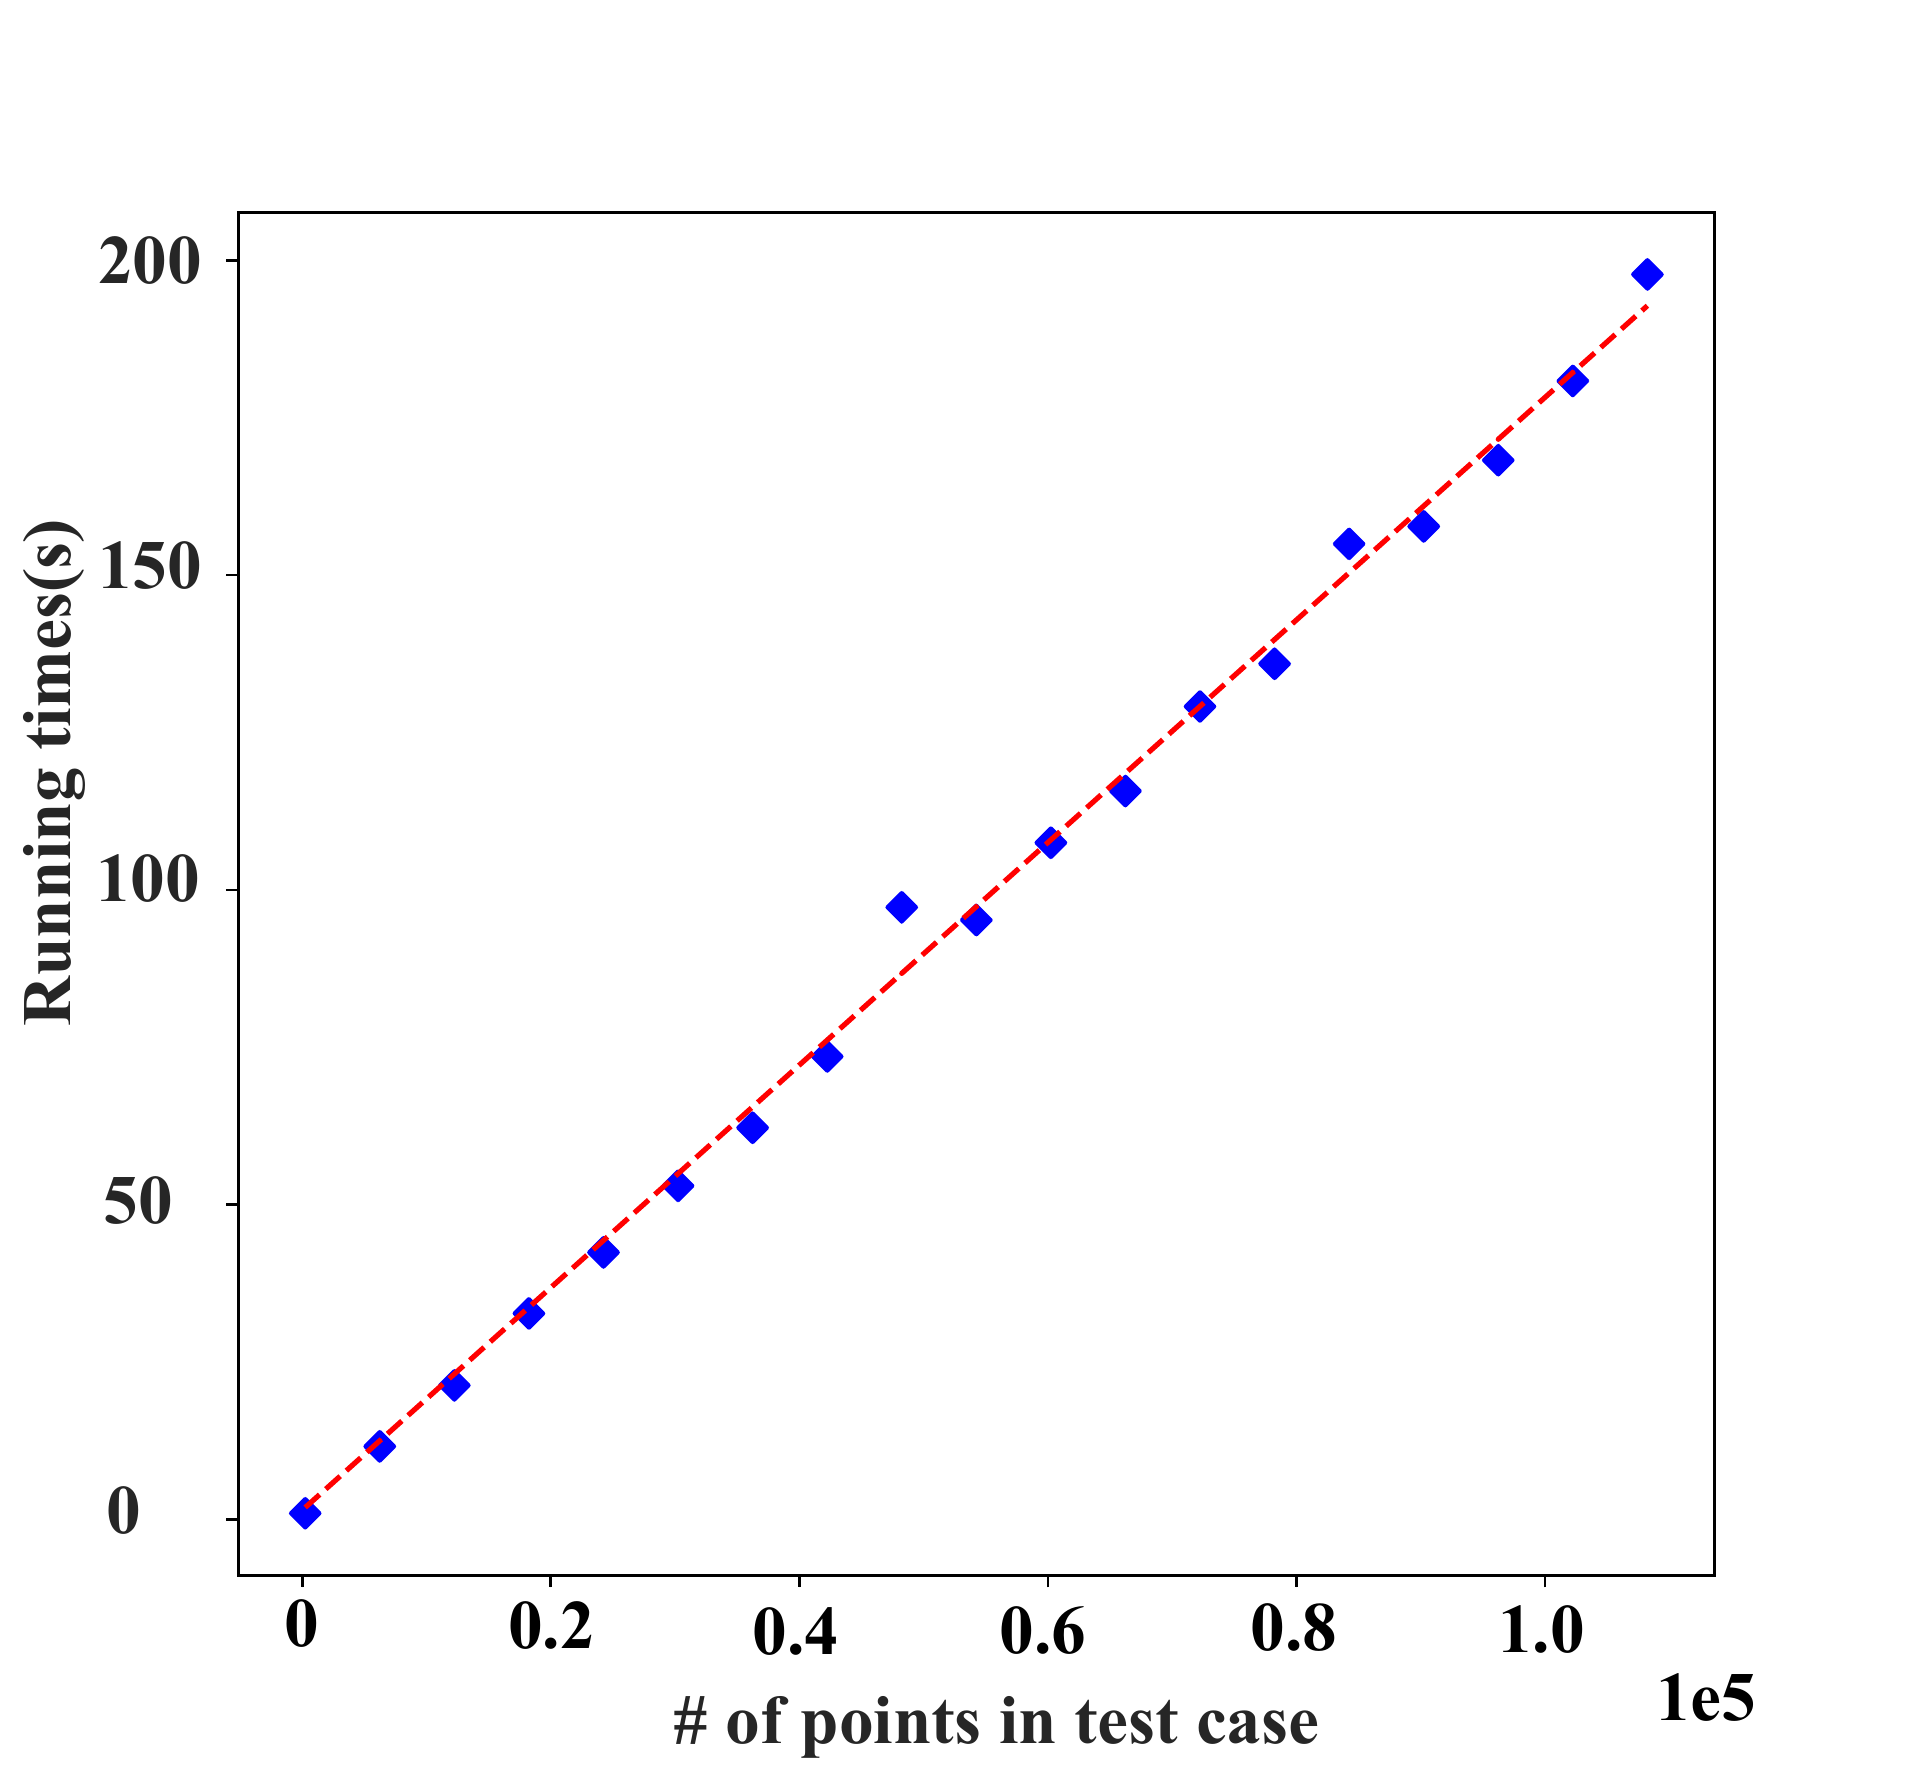}
        \end{minipage}
    }
    \subfigure[Loss curve of missgan during training. ]{
        \label{fig:lossgd}
        \begin{minipage}{0.3\linewidth}
            \includegraphics[width=\linewidth]{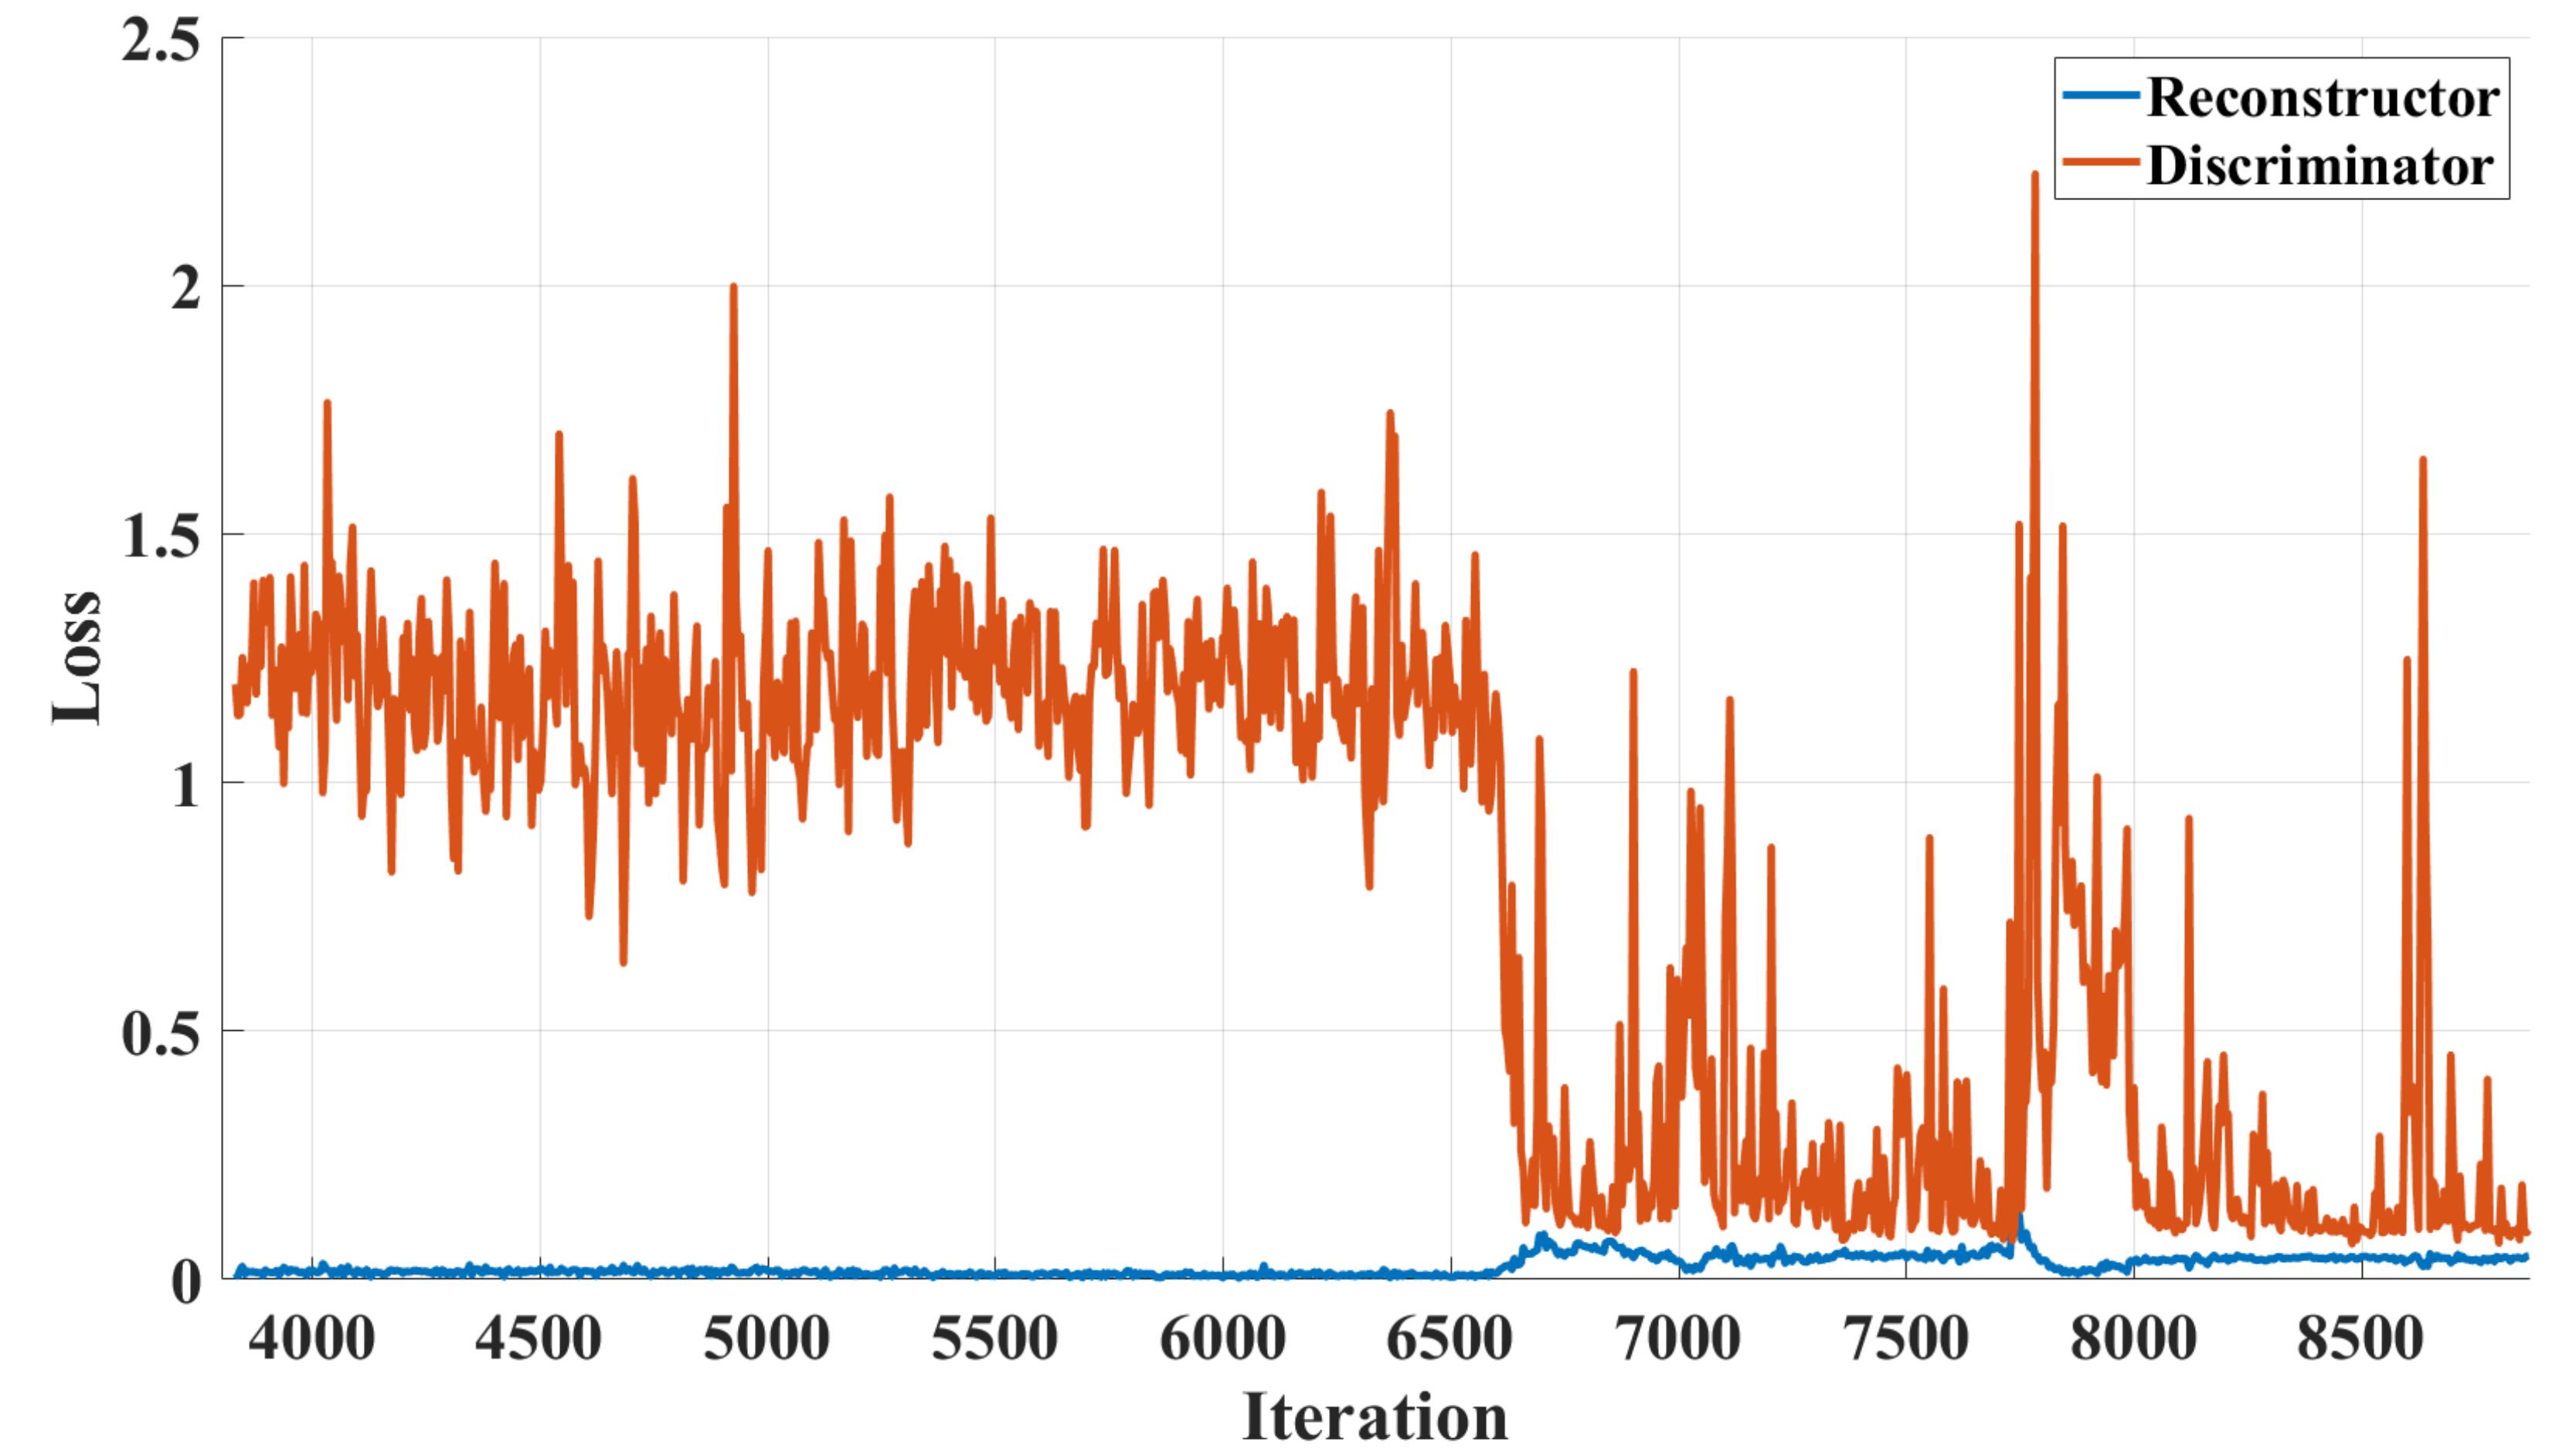}
        \end{minipage}
    }
    \subfigure[Loss curve of validation set during training.]{
        \label{fig:lossval}
        \begin{minipage}{0.3\linewidth}
            \includegraphics[width=\linewidth]{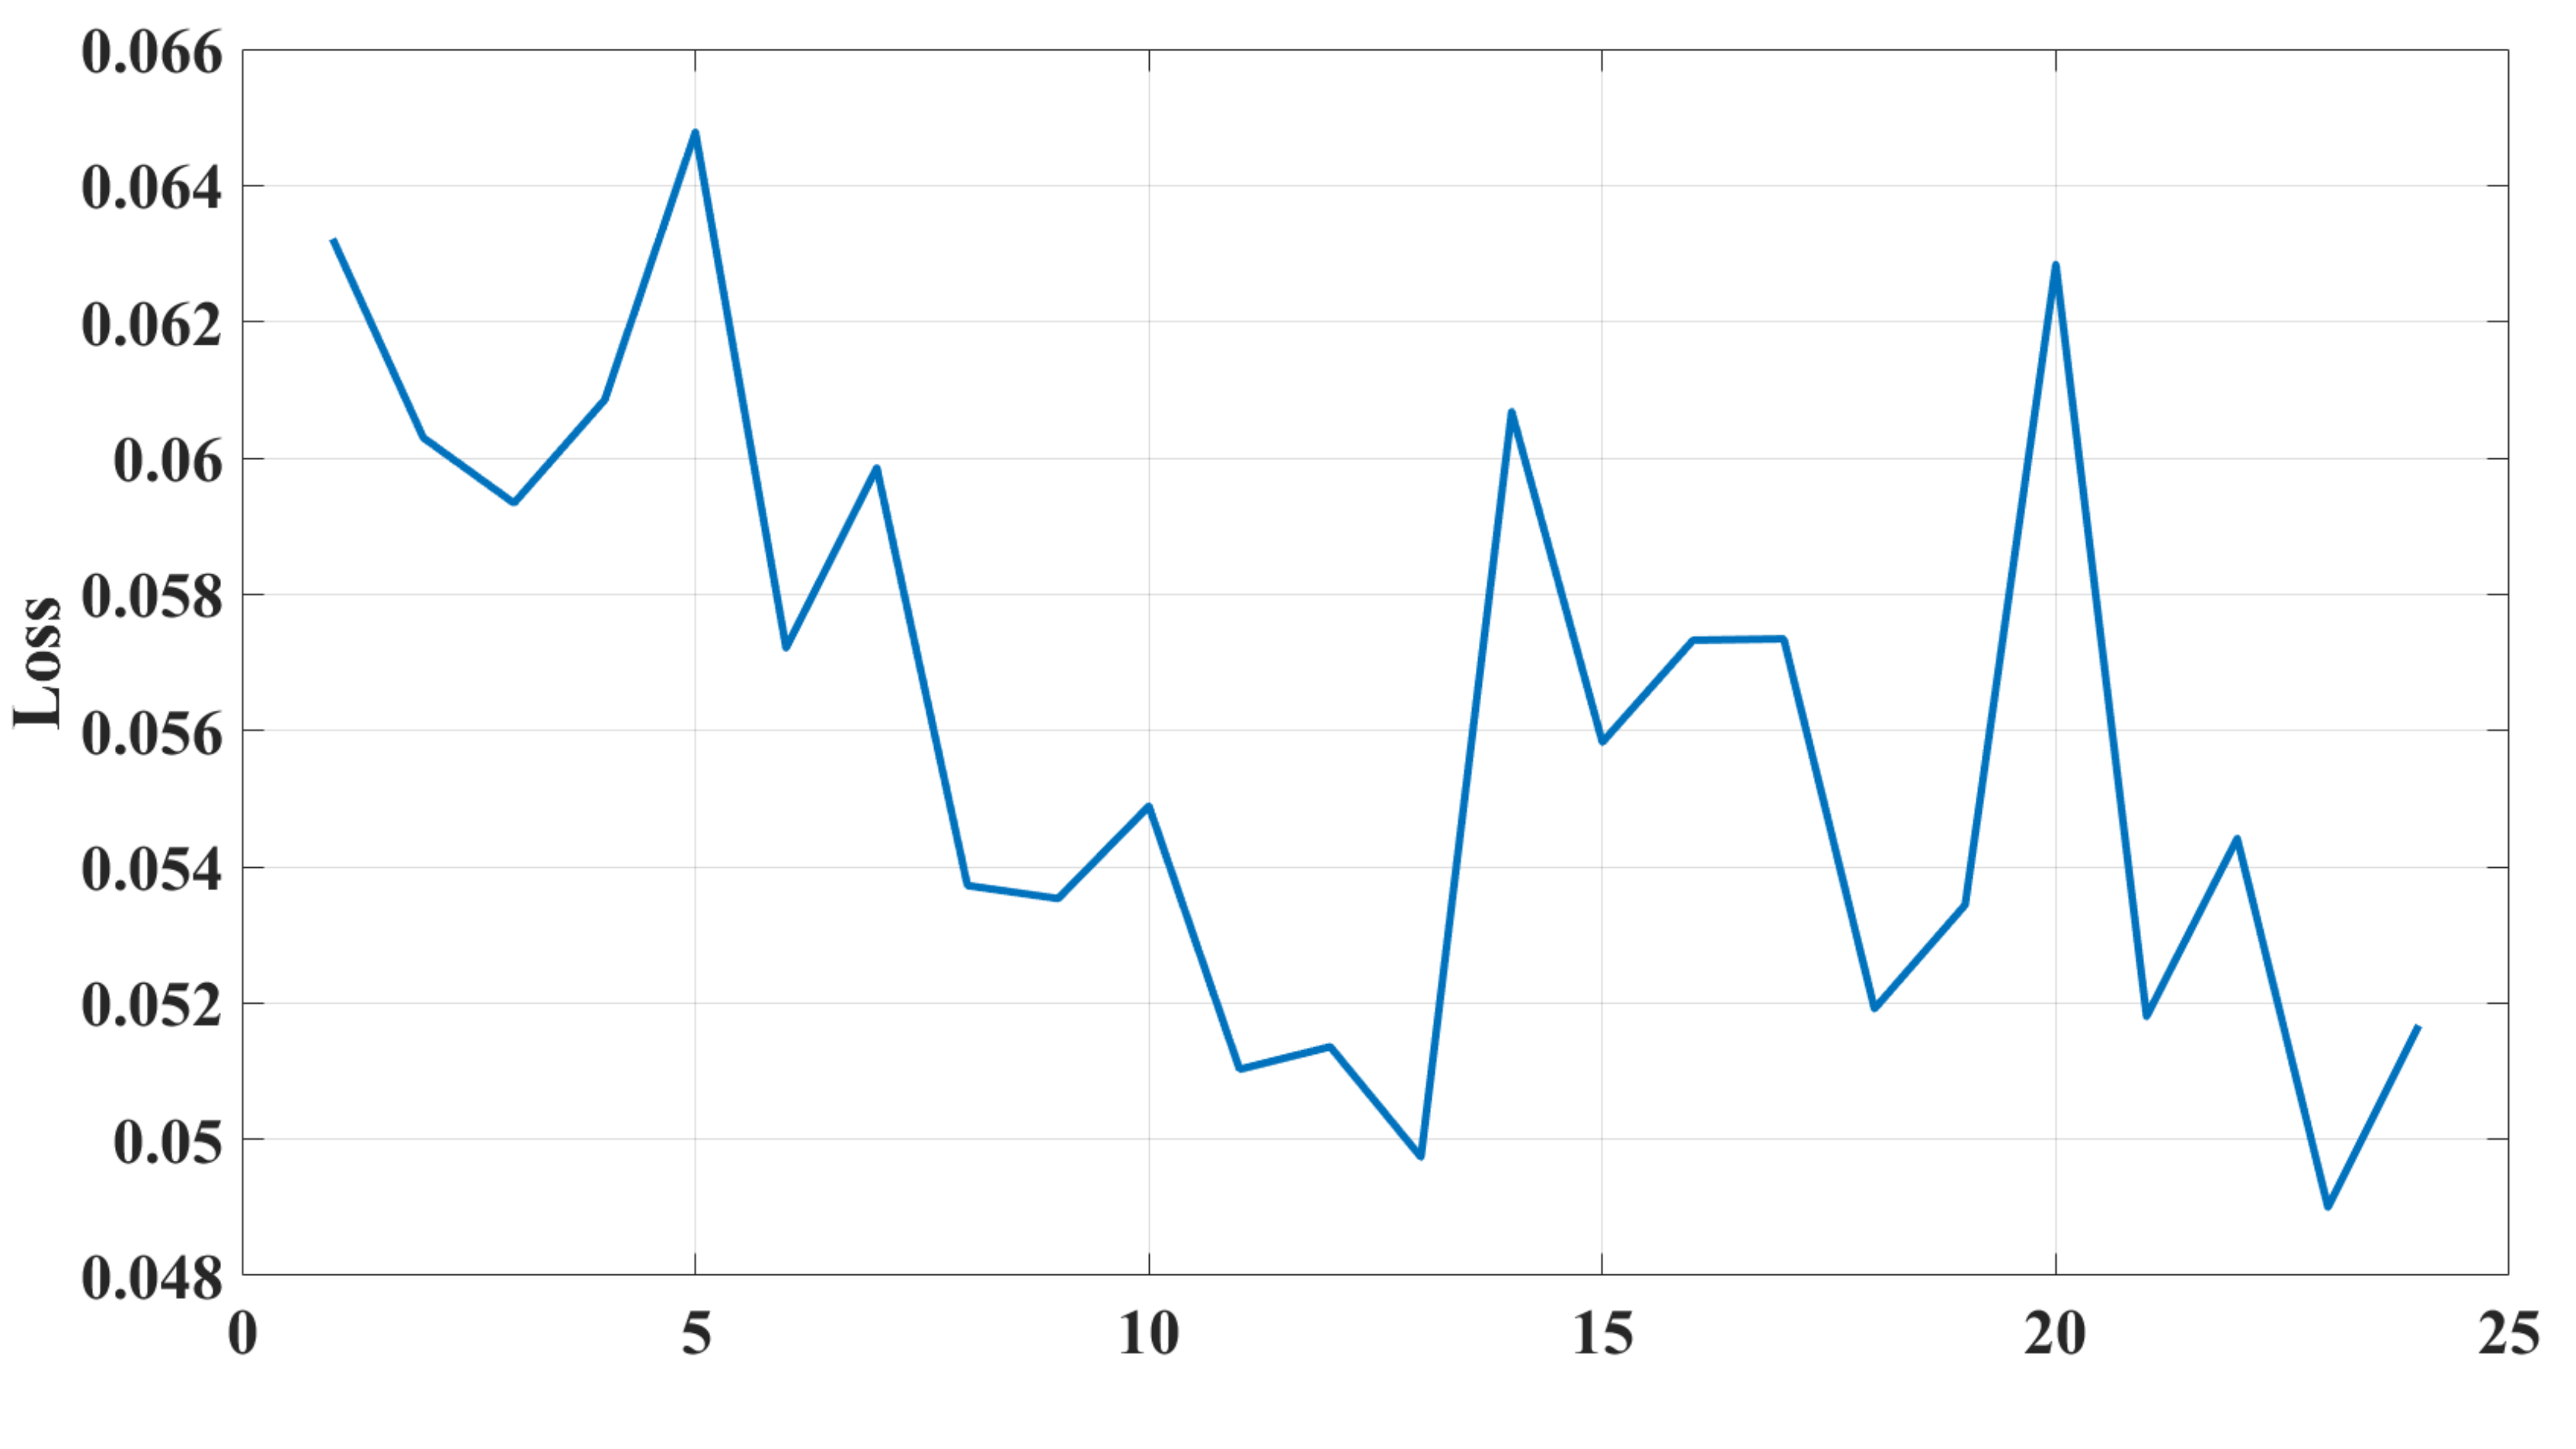}
        \end{minipage}
    }
    \caption{
        (a). Results display linear relation of running time
        and number of points which shows the scalability of \method.
        (b). Blue line stands for loss of reconstructor while orange line refers to loss of discriminator.
        (c). Test on validation set is made after each epoch of training.
    }
\end{figure*}

\atnn{Fig~\ref{fig:lossgd} demonstrates change of loss during training. From the curve we can see the deviation of loss which points out the difficulty
    of training a GAN. However, with the help of conditional information, loss of reconstructor is quite low during the whole process.
    Furthermore, after adequate iterations of training, loss of discriminator declines observably. Fig~\ref{fig:lossval} depicts curve of
    loss on validation set during training. Rapid drop happens after the fifth time of testing on validation set. Final result is rather small compared with
    the initial value.}
